# Supplementary material for: GLoRE: Evaluating Logical Reasoning of Large Language Models
Source: arXiv:2310.09107 source file (2025-04-20)
Supplement: Supplementary file 1 [file C-appendix.tex]

%% \section{Appendix}

\section{Datasets Examples}
\label{sec:appendix_a}
We illustrate data examples mentioned in Section~\ref{sec:data} here.

Figure \ref{fig:logiqa} is an example from the LogiQA 2.0 test set.
In this example, investigators want to certify the connection between astrological signs and personality. However, the volunteers who attended the program were biased because introverted people are less likely to attend such investigations. This fact flaws the conclusion of the investigation.

\begin{figure}[htbp]
\centering
\setlength{\abovecaptionskip}{0.1cm}
\setlength{\belowcaptionskip}{0.2cm}
\includegraphics[width=0.48\textwidth]{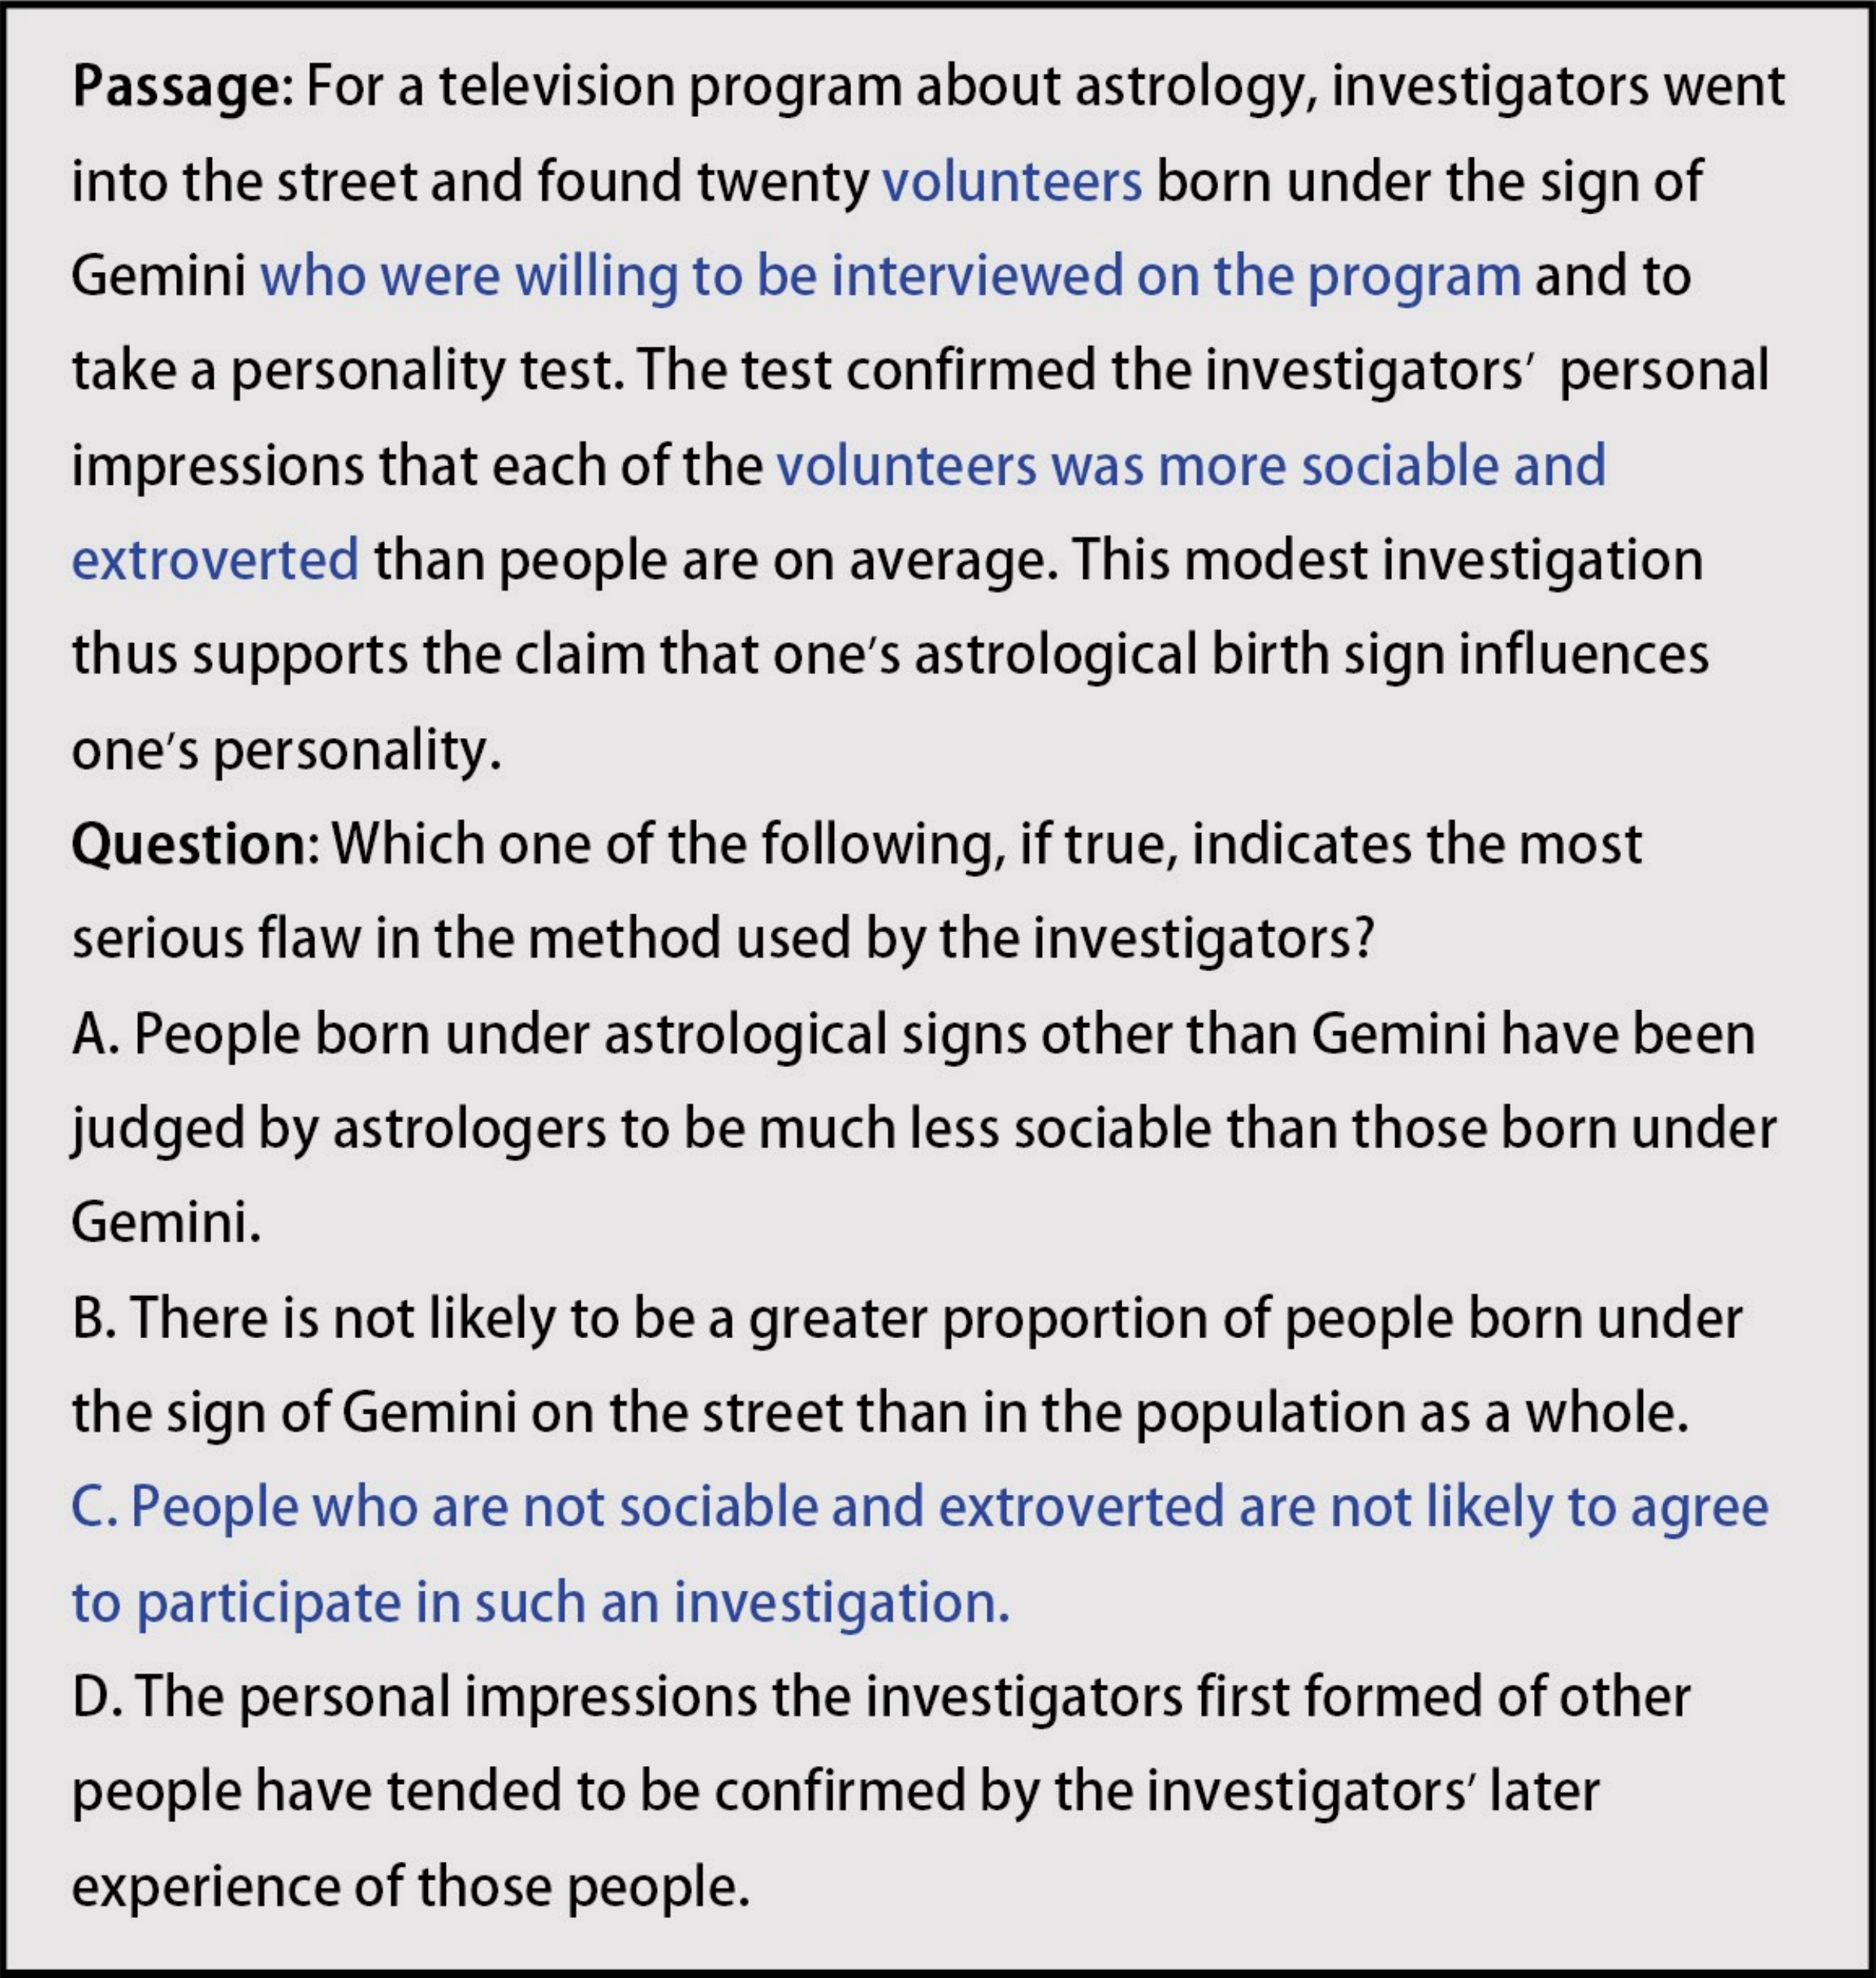}
\caption{A multi-choice reading comprehension example from the LogiQA 2.0 dataset. }
\label{fig:logiqa}
%\vspace{-0.5cm}
\end{figure}

\begin{figure}[htbp]
\centering
\setlength{\abovecaptionskip}{0.1cm}
\setlength{\belowcaptionskip}{0.2cm}
\includegraphics[width=0.48\textwidth]{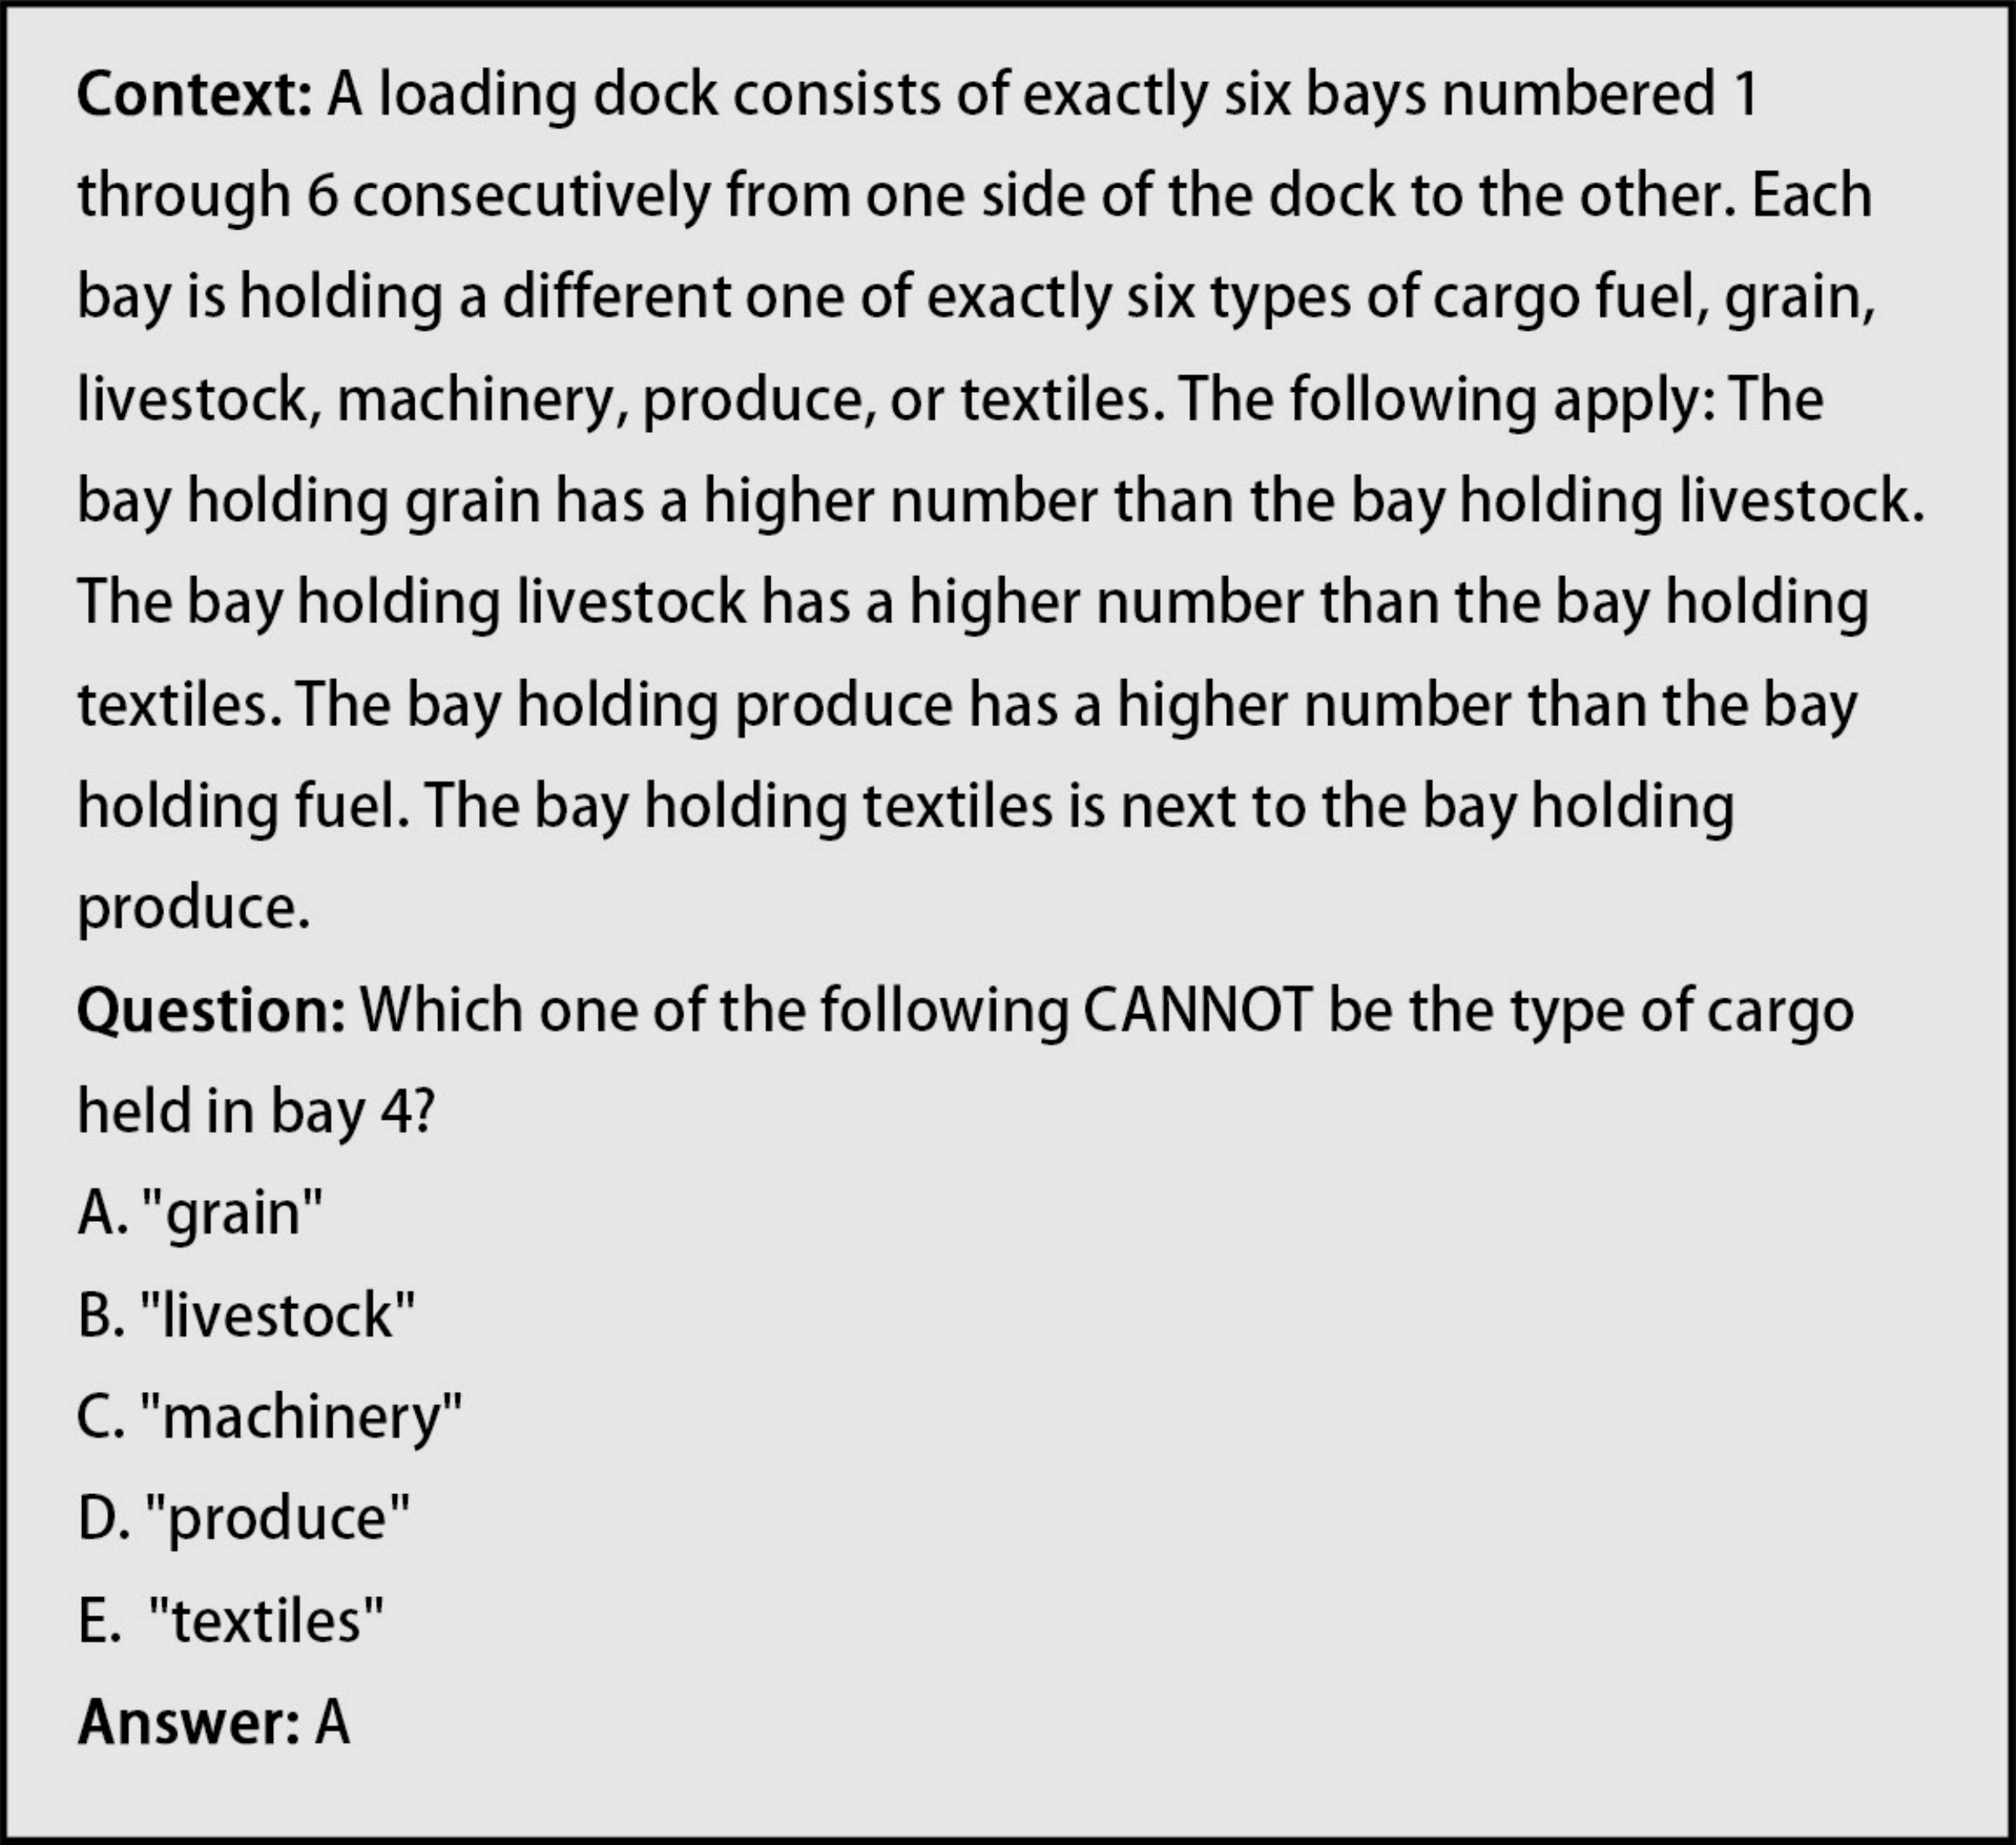}
\caption{An example from the AR-LSAT dataset.  }
\label{fig:arlsat}
%\vspace{-0.5cm}
\end{figure} 

\begin{figure}[htbp]
\centering
\setlength{\abovecaptionskip}{0.1cm}
\setlength{\belowcaptionskip}{0.2cm}
\includegraphics[width=0.48\textwidth]{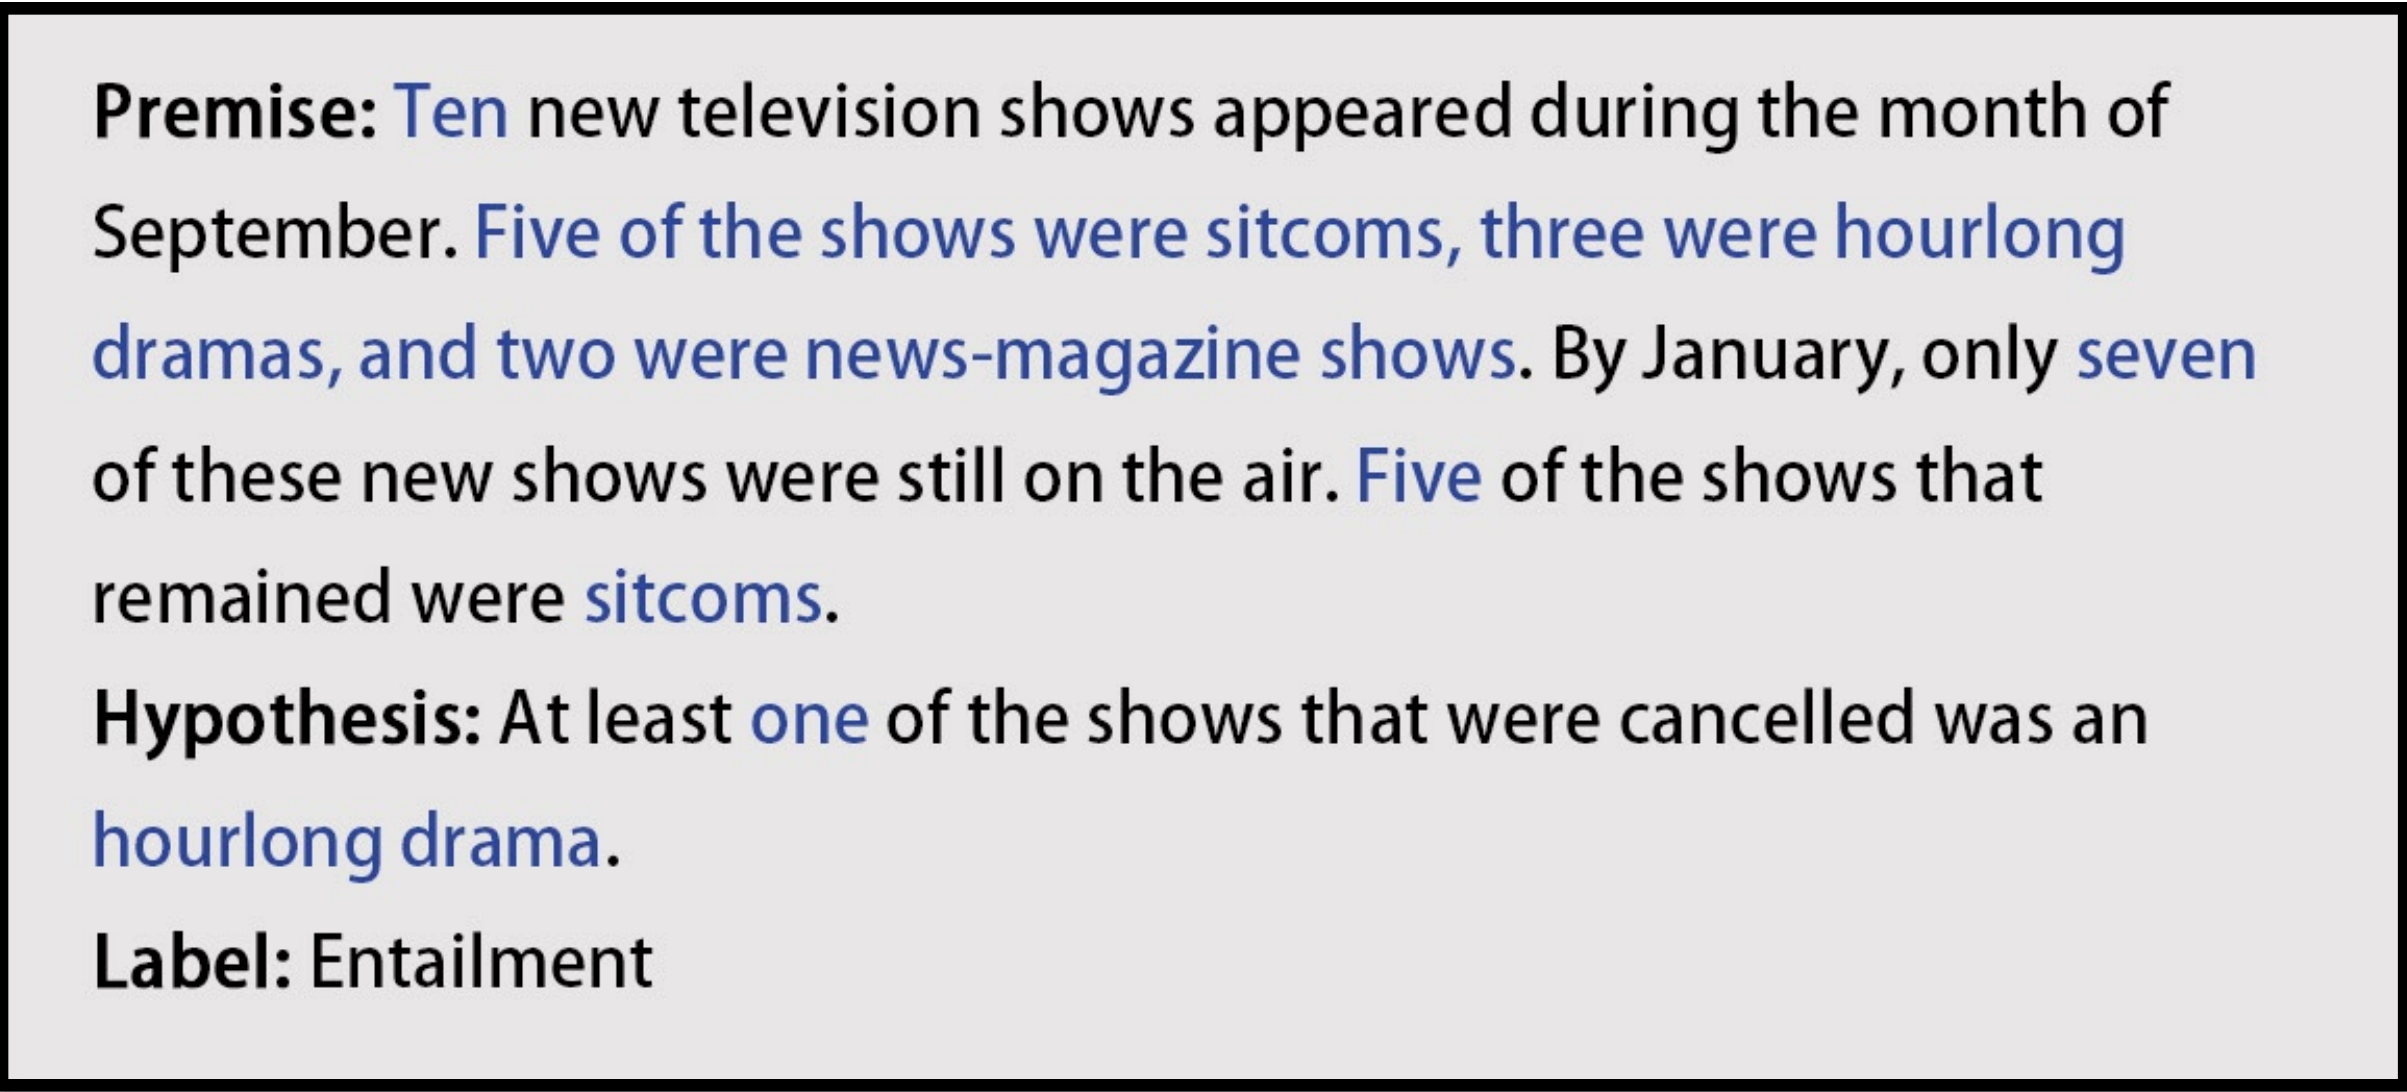}
\caption{An NLI example from the ConTRoL dataset.}
\label{fig:control}
%\vspace{-0.5cm}
\end{figure} 

\begin{figure}[htbp]
\centering
\setlength{\abovecaptionskip}{0.1cm}
\setlength{\belowcaptionskip}{0.2cm}
\includegraphics[width=0.48\textwidth]{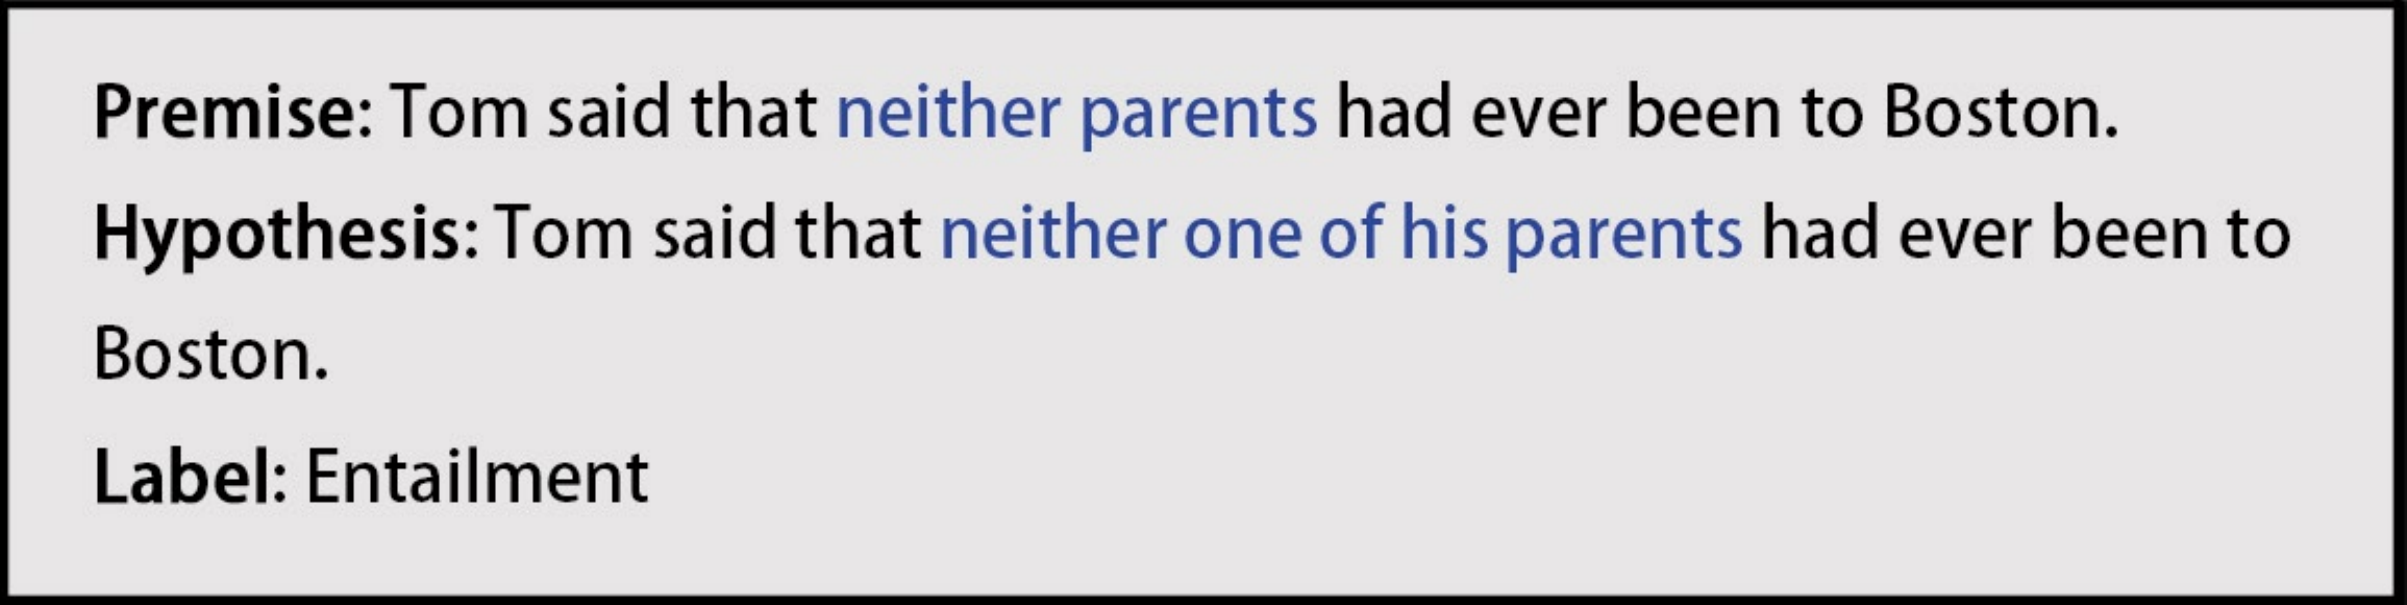}
\caption{An NLI example from the HELP dataset.}
\label{fig:help}
%\vspace{-0.5cm}
\end{figure}

\begin{figure}[htbp]
\centering
\setlength{\abovecaptionskip}{0.1cm}
\setlength{\belowcaptionskip}{0.2cm}
\includegraphics[width=0.48\textwidth]{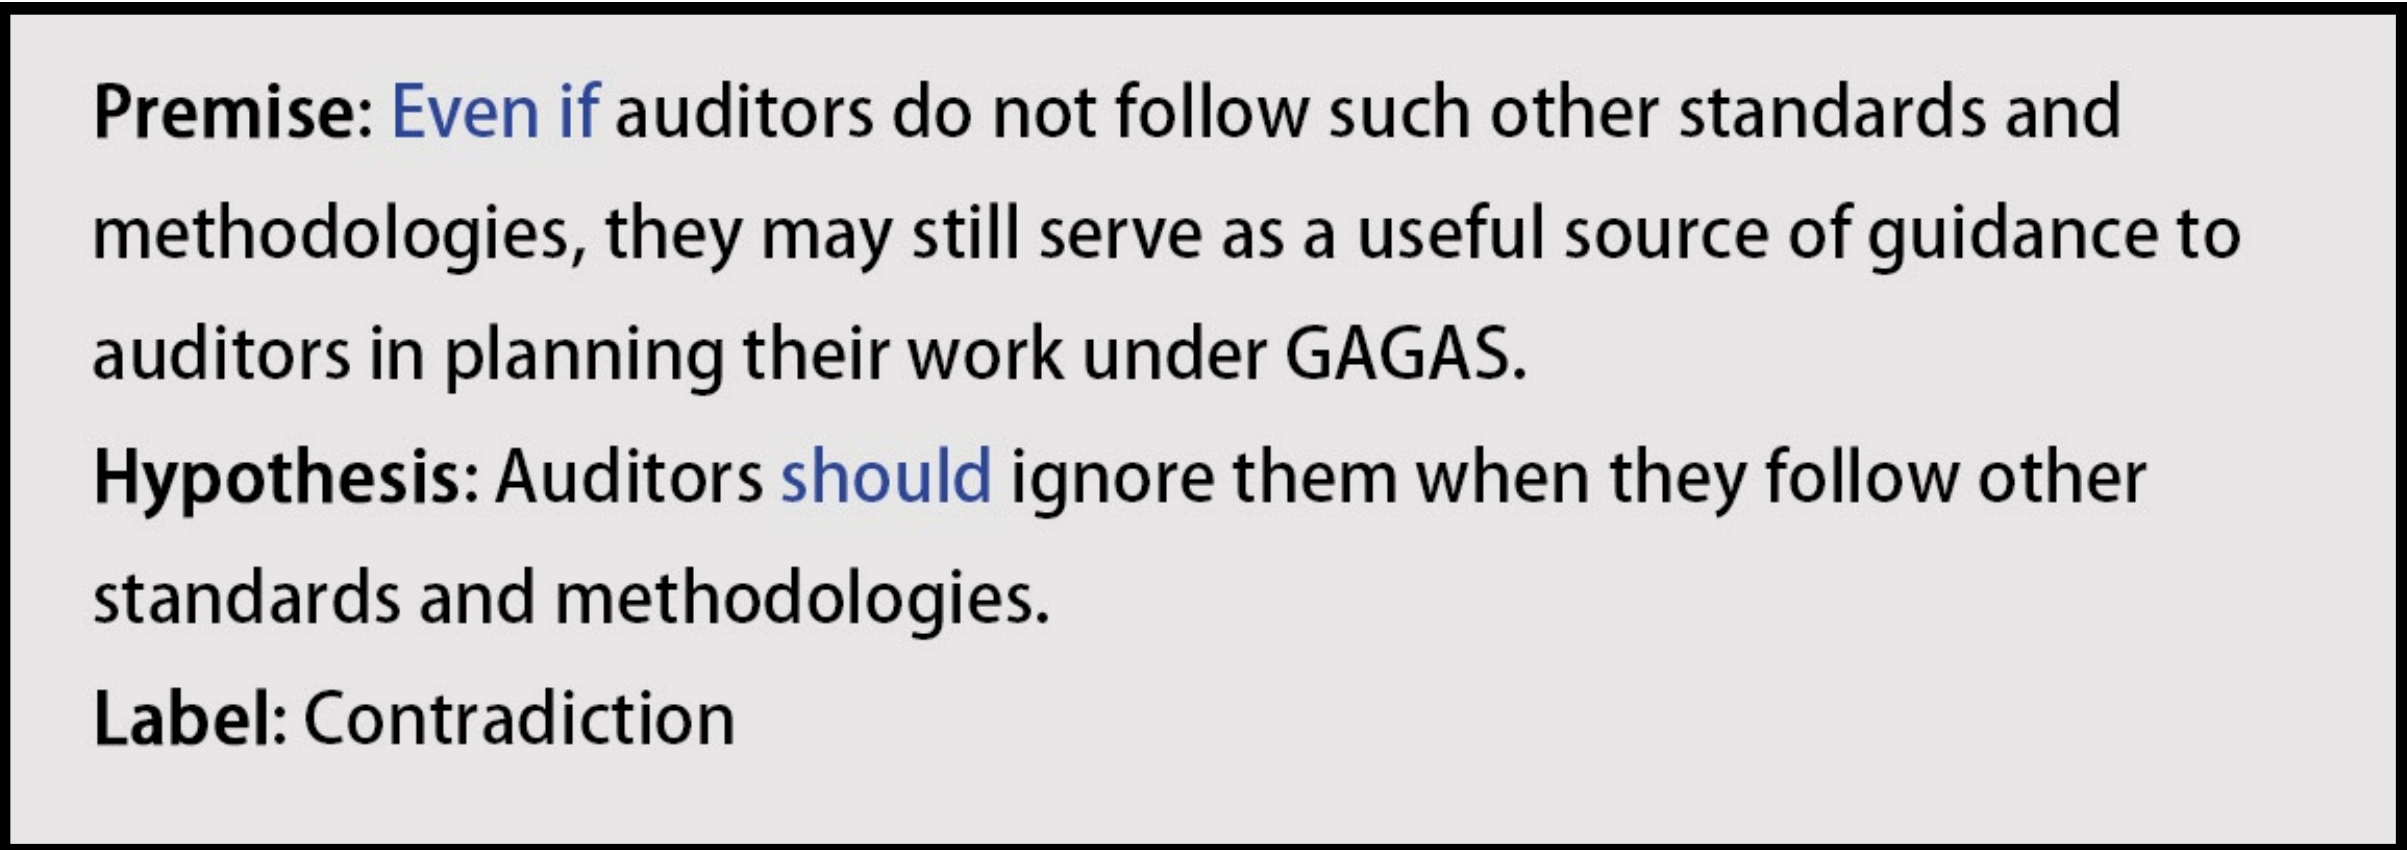}
\caption{An NLI example from the TaxiNLI dataset.}
\label{fig:taxinli}
%\vspace{-0.5cm}
\end{figure}

\begin{figure}[htbp]
\centering
\setlength{\abovecaptionskip}{0.1cm}
\setlength{\belowcaptionskip}{0.2cm}
\includegraphics[width=0.48\textwidth]{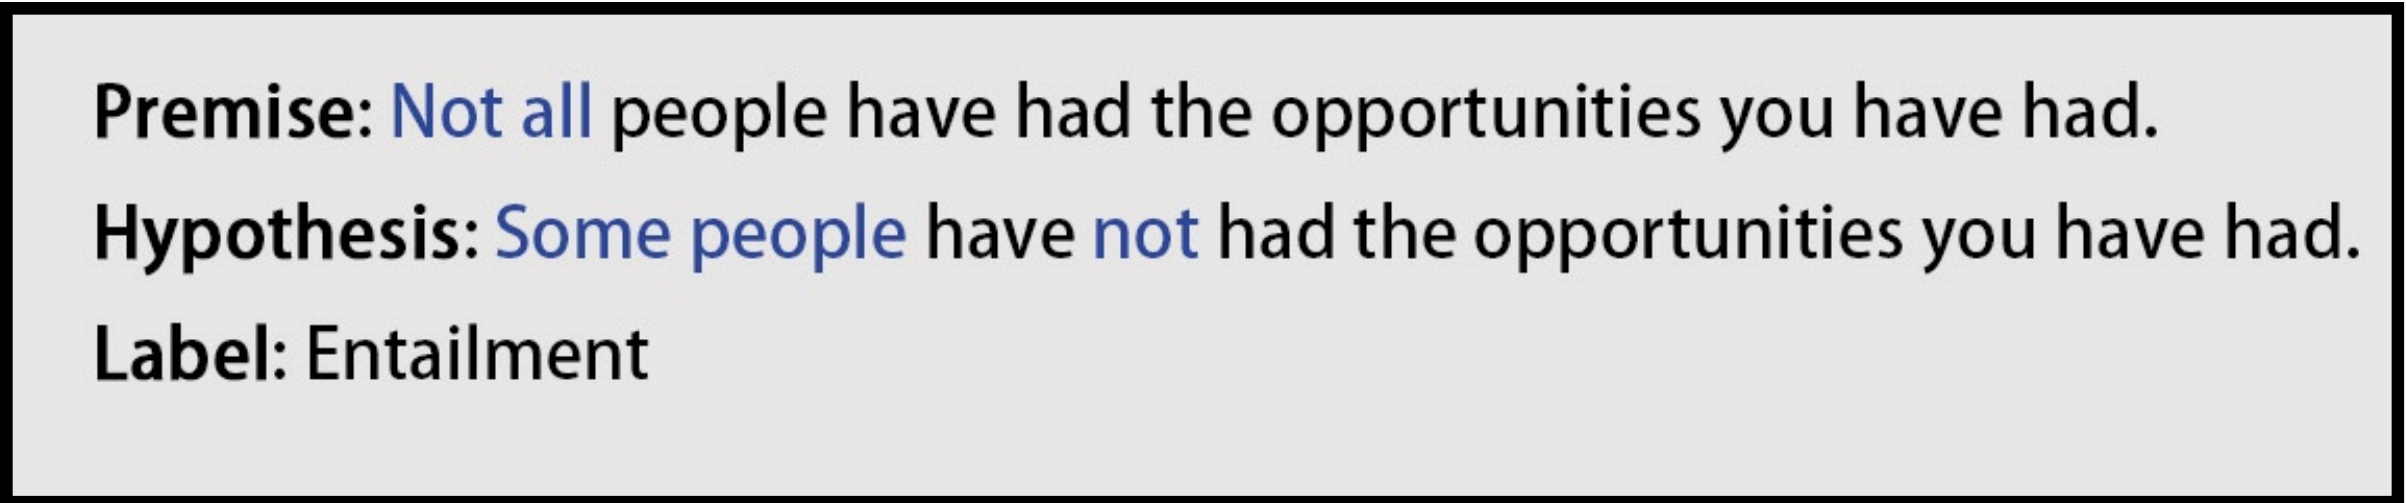}
\caption{An NLI example from the NAN-NLI dataset.}
\label{fig:nannli}
%\vspace{-0.5cm}
\end{figure}

\begin{figure}[htbp]
\centering
\setlength{\abovecaptionskip}{0.1cm}
\setlength{\belowcaptionskip}{0.2cm}
\includegraphics[width=0.48\textwidth]{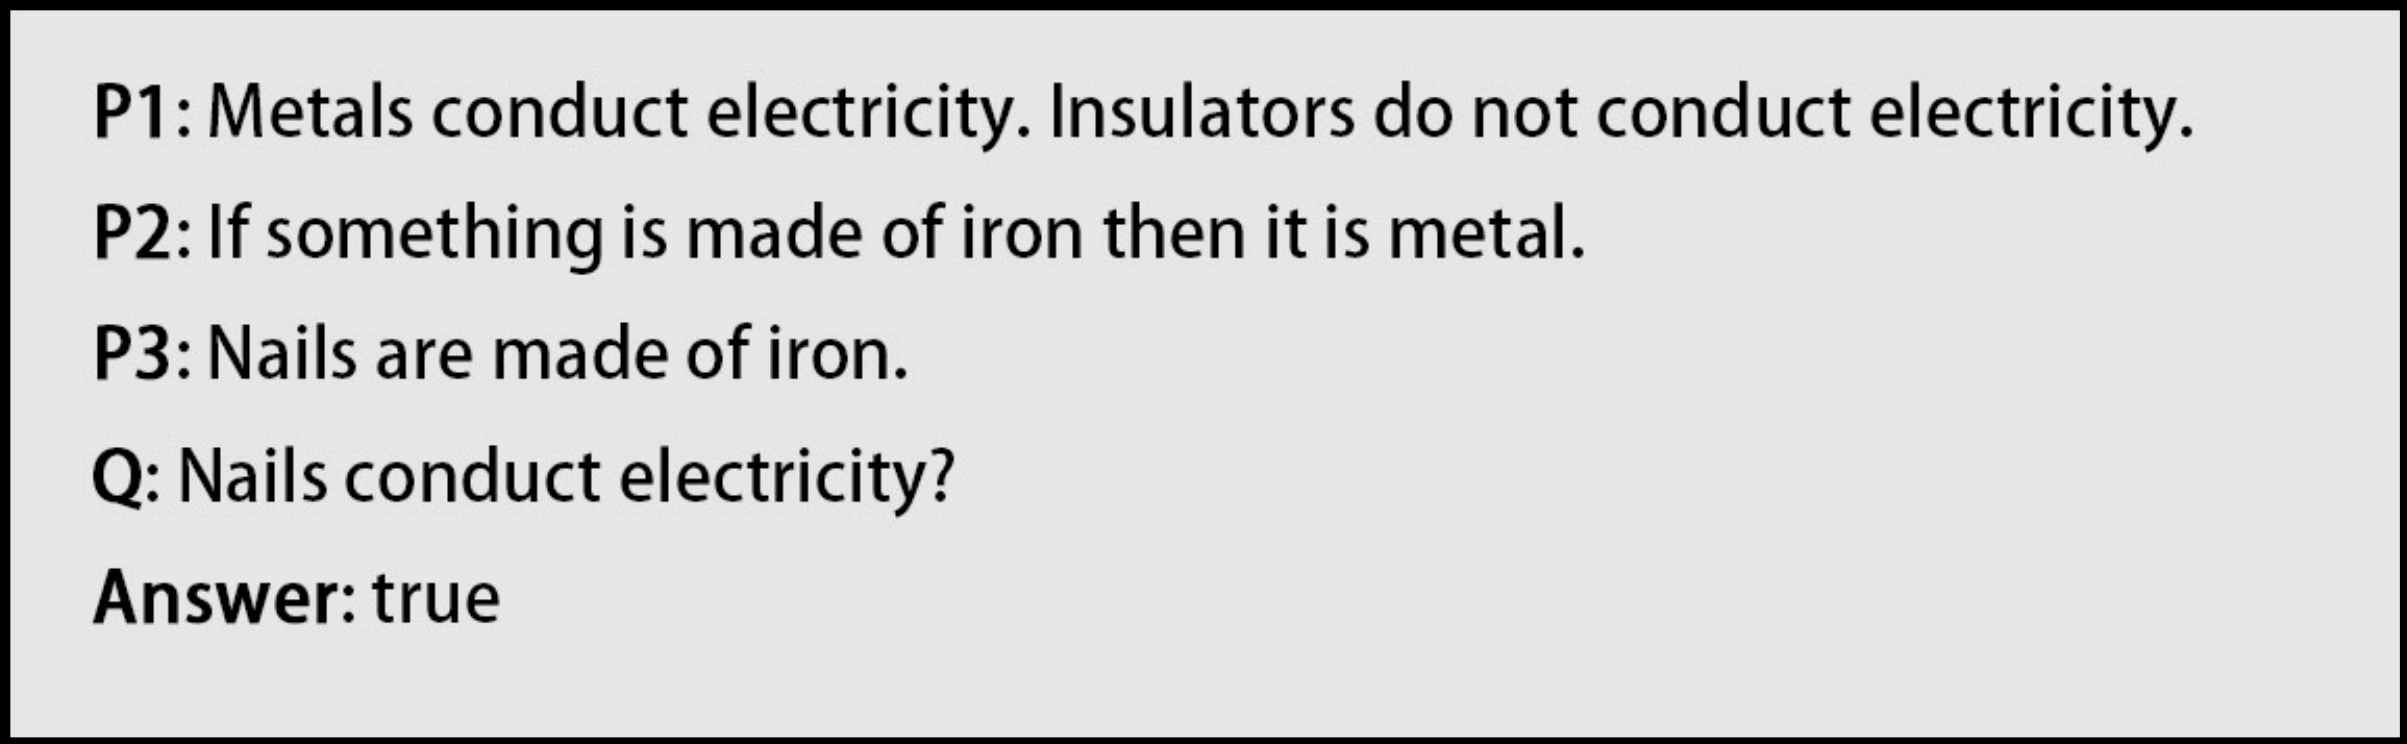}
\caption{An example from the RuleTaker dataset.}
\label{fig:ruletaker}
%\vspace{-0.5cm}
\end{figure}

\begin{figure}[htbp]
\centering
\setlength{\abovecaptionskip}{0.1cm}
\setlength{\belowcaptionskip}{0.2cm}
\includegraphics[width=0.48\textwidth]{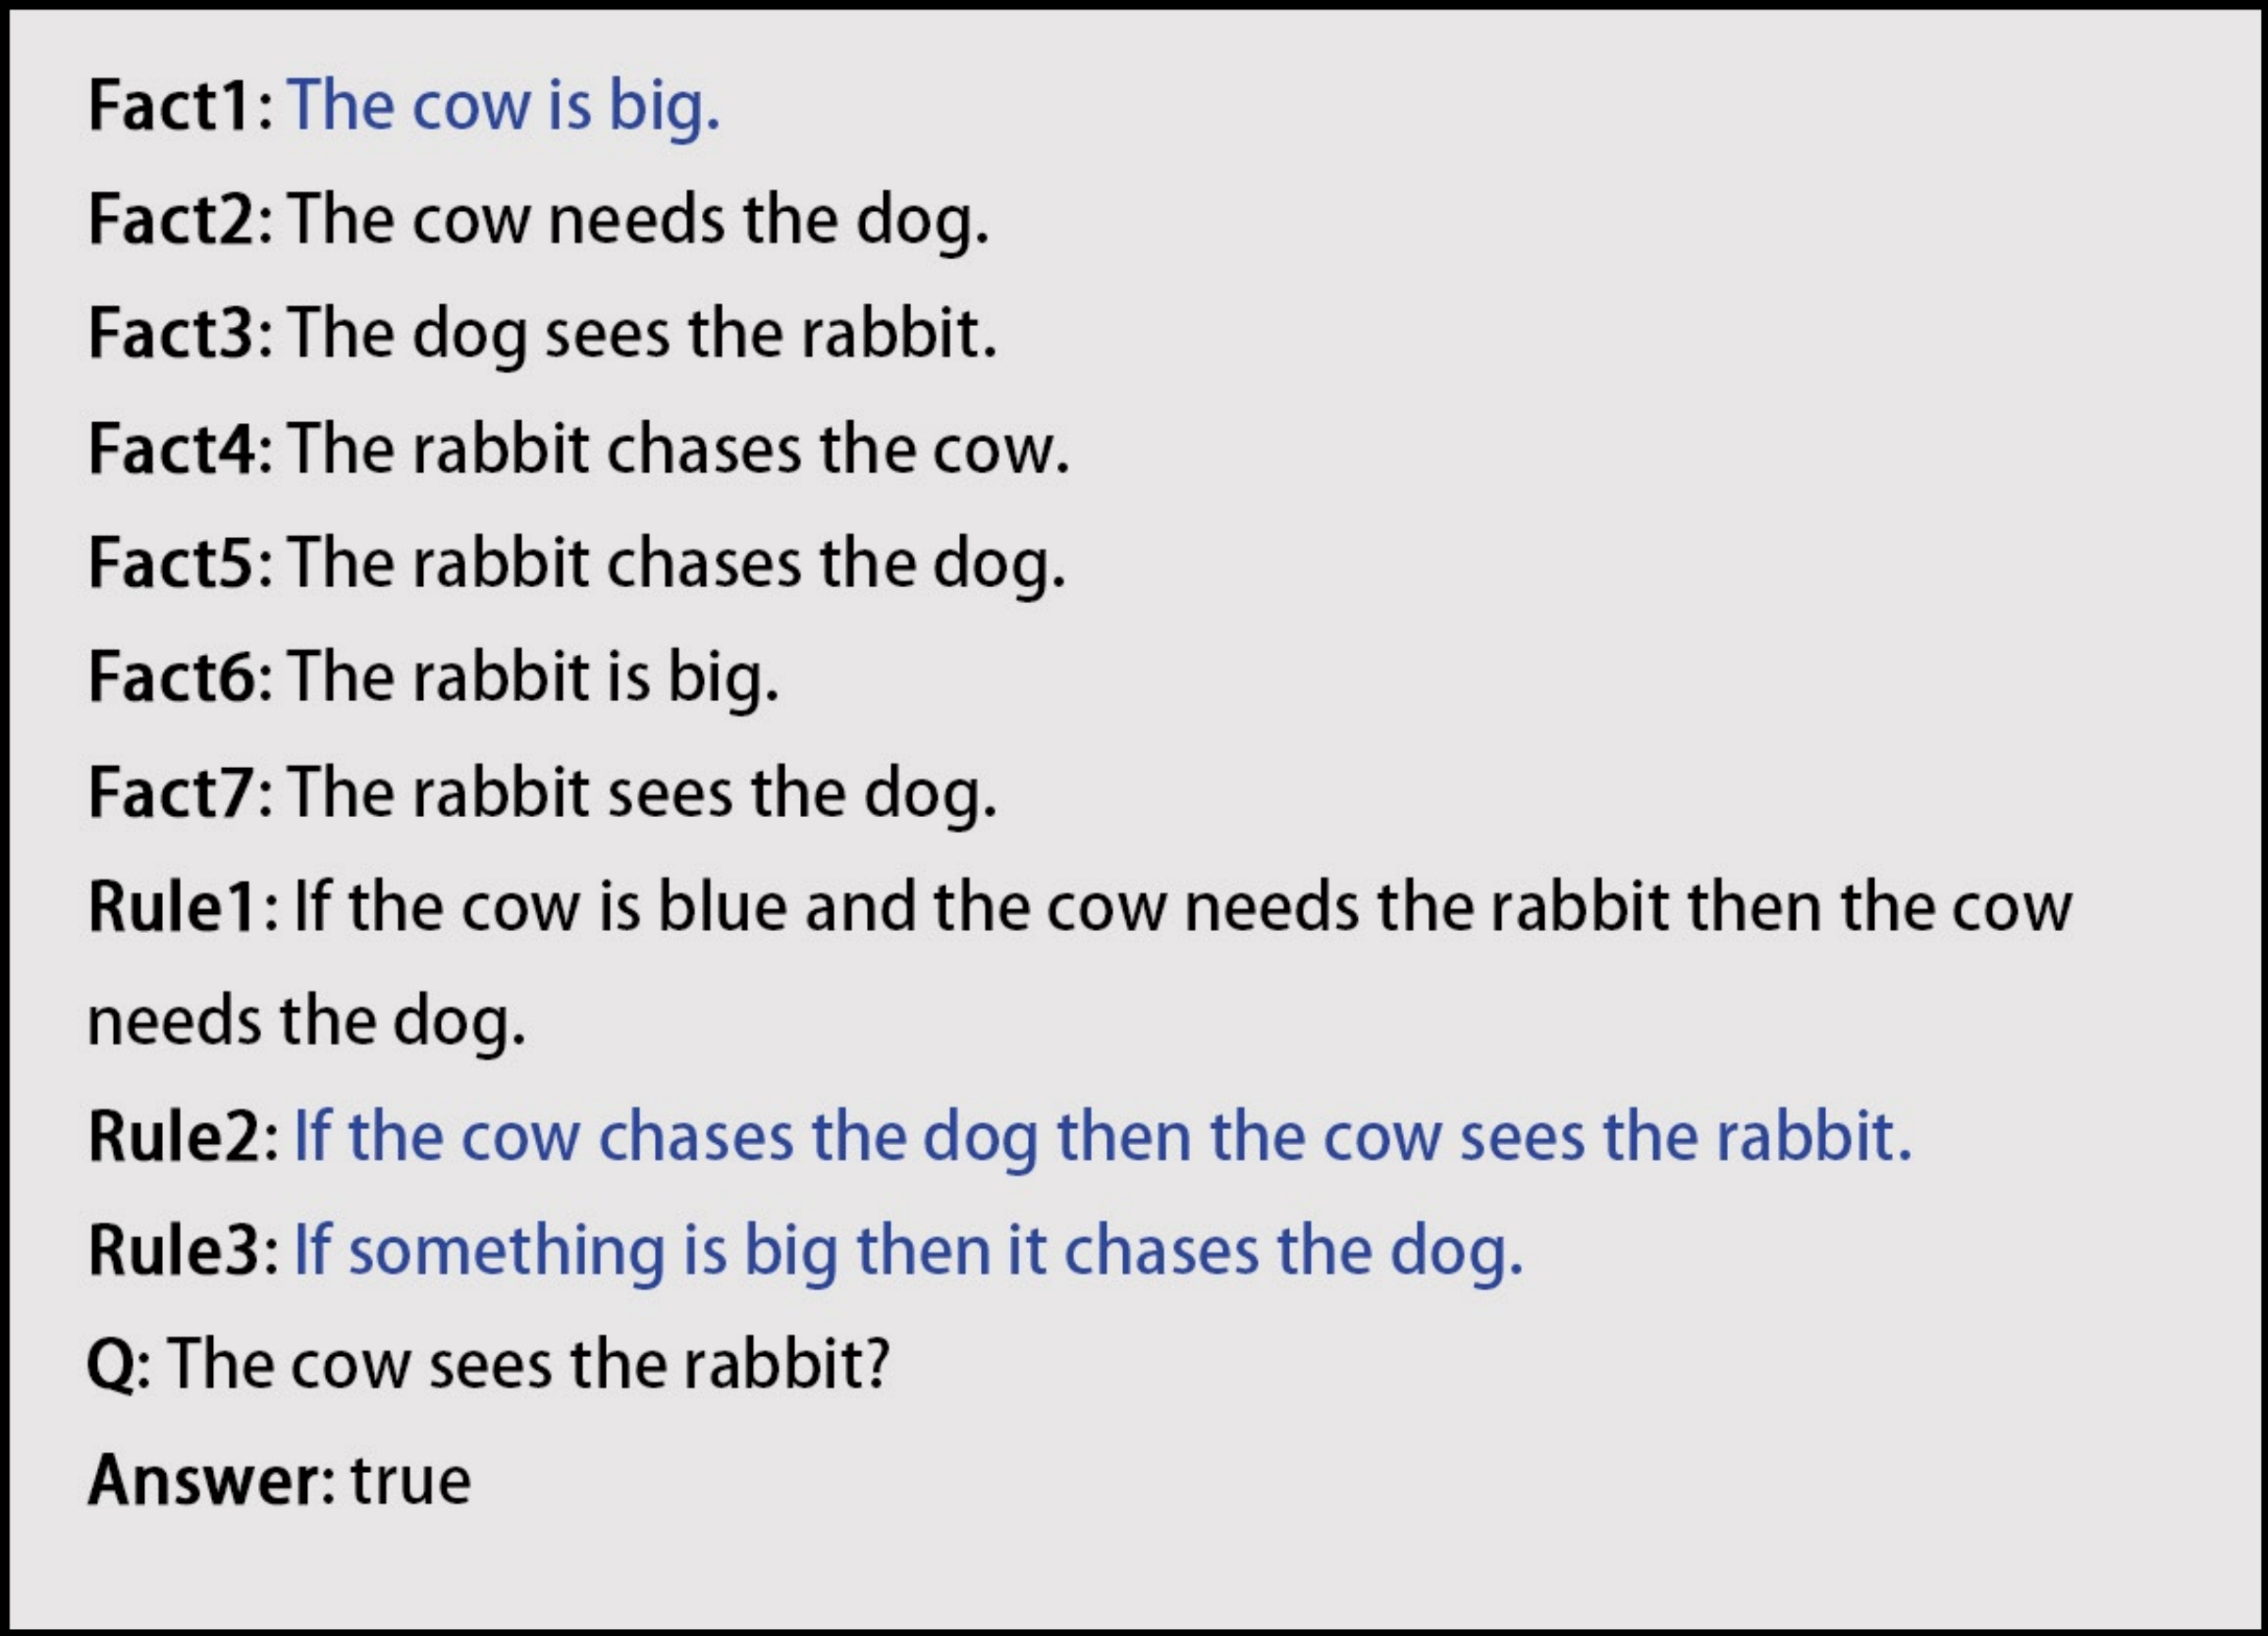}
\caption{An example from the ProofWriter dataset.  }
\label{fig:proofwriter}
%\vspace{-0.5cm}
\end{figure}
